# Supplementary material for: Attentive Multi-Layer Perceptron for Non-autoregressive Generation
Source: arXiv:2310.09512 source file (2023-10-14)
Supplement: Supplementary file 1 [file 06_appendix.tex]

\section{AR-based AMLP}
\label{sec:why_not_ar_amlp}
We here present the detailed reason why we do not fuse AMLP with AR models.

\paragraph{\hl{AMLP is not suitable for AR}}
In AR models, the self/cross attention is different from NAR models and they require to maintain causality due to teacher forcing training. 
To enable causal (decoder) AMLP, the overall time consumption and memory costs in the training phase are hugely increased. 
Such drawback is also revealed in most efficient attention (like Nystr\"omformer~\citep{xiong2021nystromformer}, Local, cosFormer~\citep{qin2022cosformer}, Performer~\citep{choromanski2020rethinking}) that also adopt softmax kernel decomposition for speed-up. 
To replace decoder self attention, they also need to pay extra complexity during training~\citep{RFA}. 
Therefore, these efficient attention and AMLP are also not straightforward to be adopted for AR models. 
\paragraph{\hl{AMLP suits NAR}}

In contrast to AR models where typical efficient models and AMLP all suffer from inefficiency, the training objective and identically independent distribution~(i.i.d.) assumption of NAR models avoid teacher forcing.
NAR thus suits the application of efficient attention and AMLP. 
As a result, AMLP is dedicated to NAR models for even higher efficiency in both training and inference.

\paragraph{Example of AR-AMLP}
We present the specific computation steps of AMLP in AR scenario and explain the drawbacks of AR-AMLP.
We take \amlpone~as an example.
Given an query token $\boldsymbol{q}_t$, the covariances $\mathbf{S}_t^{\mathbf{Q}}$ and $\mathbf{S}_t^{\mathbf{K}}$ of $\mathbf{K}_{t}$ and $\mathbf{Q}_{t}$, and the cross-covariance $\mathbf{z}_t$ of $\mathbf{K}_t$ and $\mathbf{V}_t$, $W_{\mathbf{Q,K}}$ and $W_\mathbf{{\mathbf{Q,K,V}}}$ are formulated as follows:
\begin{align}
    \label{eq:causal_weight}
    W_{\mathbf{Q}_{t},\mathbf{K}_t}=\mathbf{L}_t^\top&=C_q(\sigma_2(\mathbf{S}_t^{\mathbf{Q}}))+C_k(\sigma_2(\mathbf{S}_t^{\mathbf{K}})) \\
    W_{\mathbf{Q}_{t},\mathbf{K}_t, \mathbf{V}_t}&=\mathbf{L}_t^\top\sigma_2(\mathbf{z}_t)
\end{align}
where $\mathbf{S}_t^{\mathbf{Q}}=\mathbf{S}_{t-1}^{\mathbf{Q}}+\boldsymbol{q}_t^\top\boldsymbol{q}_t$, $\mathbf{S}_t^{\mathbf{K}}=\mathbf{S}_{t-1}^{\mathbf{K}}+\boldsymbol{k}_t^\top\boldsymbol{k}_t$ and $\mathbf{z}_t=\mathbf{z}_{t-1}+\boldsymbol{k}_t^\top\boldsymbol{v}_t$.
These computation steps increase heavy memory costs and large time consumption in the training phase, with an additional $O(ncd)$ costs beyond the overall computation.
Recurrent computation also harms the parallelism and further slows down the training process.

\section{From Attention to AMLP}
\label{sec:from_attn_to_amlp}
\hl{We here show that AMLP fuses attentive ability through kernel function approximation, matrix decomposition and reformulation. }

1. In vanilla attention, $\mathrm{softmax}(QK^\top)$ is a softmax kernel which can be decomposed into a multiplication of two kernel functions: $\phi(Q)\cdot\phi(K)^\top$, which is verified in Performer~\citep{choromanski2020rethinking}, cosFormer~\citep{qin2022cosformer} and LARA~\citep{lara}. 
Hence, we here use a distance matrix $\Sigma$ to serve as a bridge which enables $Q\Sigma K^\top$ to be decomposed with fewer eigenspectrums like Performer.

2. The low rank approximation of the attention matrix, $\mathrm{softmax}(QK^\top)$,  does not impact the performance much, which is verified by Nystr\"omformer~\citep{xiong2021nystromformer}. 
Based on their findings, the kernel function $Q\Sigma K^\top$ can also enjoy lower computation costs from low rank approximation.

3. Combined with two results, AMLP reformulates the attention $\mathrm{softmax}(QK^\top)$ with $Q\Sigma K^\top$ and uses Nystrom's findings to decompose $\Sigma$ into two matrices. Finally, AMLP reparameterizes the decomposed matrices and maintains the attentive functionality as $\mathrm{Attn}(Q, K, V)$.

\section{Task Description}
We provide the statistics of tasks in Table~\ref{tab:task_statistic}.

\begin{table}[htbp]
  \centering
  \caption{Task statistics of evaluation metrics, input sequence lengths and backbone neural networks. For encoder-decoder architectures, we show both source and target lengths. ($\dag$) denotes the sequence lengths of encoders and decoders of Tr-TTS. The number of final audio phonemes after the vocoder is 559 as well.}
    \begin{tabular}{lllll}
    \toprule
    \textbf{Task} & \multicolumn{1}{l}{\textbf{Dataset}} & \multicolumn{1}{l}{\textbf{Length}} & \multicolumn{1}{l}{\textbf{Model}} & \multicolumn{1}{l}{\textbf{Metric}} \\
    \midrule
    \multirow{2}[2]{*}{TTS} & \multirow{2}[2]{*}{LJSpeech} & 559   & FastSpeech~2 & \multirow{2}[2]{*}{MCD/MSD} \\
          &       & 100/141$^{\dag}$ & Transformer-TTS &  \\
    \midrule
    \multirow{2}[2]{*}{MT} & \multirow{2}[2]{*}{WMT'14 EN-DE} & \multirow{2}[2]{*}{23/21} & Transformer \& & \multirow{2}[2]{*}{BLEU} \\
          &       &       & GLAT  &  \\
    \midrule
    \multirow{2}[2]{*}{SR} &  \multirow{2}[2]{*}{FFHQ \& CelebA-HQ}  & \multirow{2}[2]{*}{16384} & \multirow{2}[2]{*}{SR3} &  \multirow{2}[2]{*}{PSNR/SSMI} \\
          &  &       &       &  \\
    \midrule
    LSTF  & ETT   & 336/720 & Informer & MSE/MAE \\
    \bottomrule
    \end{tabular}%
  \label{tab:task_statistic}%
\end{table}%

\section{Hyperparameters of Tasks}
We provide the hyperparameters of each task in Table~\ref{tab:hyperparameters}.
We adopt the same hyperparameter sets for Transformer-TTS and FastSpeech~2, which is referred from \citet{fairseq_s2s}. Following \citet{vaswani2017attention} and \citet{qian2020glancing}, we use the same hyperparameters to train Transformer-base and GLAT, respectively.
We implement Transformer-TTS, FastSpeech~2, GLAT and Transformer with fairseq~\citep{fairseq}.
In ``Evaluation Checkpoint'' of Table~\ref{tab:hyperparameters}, ``last'' denotes that we use the last saved checkpoint to test models. 
``best'' denotes that we use the best checkpoint with the lowest MCD value in the validation set for evaluation.
``average last $n$'' denotes that we create a new checkpoint whose parameters are averaged on the parameters of last $n$ ones and use this new checkpoint for performance comparison.

\section{Details of Attention}
\paragraph{Attention hyperparameters}
We provide the hyperparameters of attentions applied in different tasks in Table~\ref{tab:attn_param}. local attention has one hyperparameter \texttt{wsize} to control the number of tokens around query one to be attended. ABC has one hyperparameter \texttt{landmark} to control the size of bounded memory. AMLP has one hyperparameter \texttt{ffn\_dimension} to control the inner dimensionality. Performer has one hyperparameter \texttt{approx\_attn\_dim} to control the dimensionality of random feature matrices. For vanilla, gMLP, XCA and cosFormer, they do not adopt hyperparameters.

\paragraph{Implementation details}
We implement ABC and local attention by ourselves because we cannot find open-sourced official implementation for them.
For Performer, cosFormer, and vanilla attention, we use their official implementation and rewrite them with PyTorch~\citep{paszke2019pytorch} if necessary.
These attention implementations in PyTorch will be released in~\url{https://github.com/Anonymous}.

\section{Experimental results on ETT dataset}
We report the complete results on ETT-h1, ETT-h2 and ETT-m1 in Table~\ref{tab:ett_full}.
% Table generated by Excel2LaTeX from sheet 'Sheet1'
\begin{table}[htbp]
  \centering
  \small
  \caption{Results on ETT-h1, ETT-h1, and ETT-m1 datasets. $n,m$ are the target and source lengths.}
%     \begin{tabular}{llrrrrrr}
%     \toprule
%     \multirow{2}[4]{*}{\textbf{Complexity}} & \multirow{2}[4]{*}{\textbf{Model}} & \multicolumn{2}{c}{\textbf{ETTh1}} & \multicolumn{2}{c}{\textbf{ETTh2}} & \multicolumn{2}{c}{\textbf{ETTm1}} \\
% \cmidrule{3-8}          &       & \multicolumn{1}{c}{\textbf{MSE↓}} & \multicolumn{1}{c}{\textbf{MAE↓}} & \multicolumn{1}{c}{\textbf{MSE↓}} & \multicolumn{1}{c}{\textbf{MAE↓}} & \multicolumn{1}{c}{\textbf{MSE↓}} & \multicolumn{1}{c}{\textbf{MAE↓}} \\
%     \midrule
%     $O(n^2+nm)$ & \textcolor[rgb]{ .122,  .137,  .161}{vanilla} & 1.257 & 0.905 & 3.548 & 1.652 & 1.028 & 0.813 \\
%     \midrule
%     \multirow{4}[4]{*}{$O(n+m)$} & ABC   & 1.332 & 0.934 & 3.430 & 1.585 & 1.037 & \textbf{0.784} \\
%     \multicolumn{1}{l}{} & Performer & 1.455 & 0.966 & 4.018 & 1.770 & 1.203 & 0.832 \\
%           & cosFormer & 1.384 & 0.963 & 3.912 & 1.707 & 1.021 & 0.792 \\
%          & AMLP  & \textbf{1.247} & \textbf{0.894} & \textbf{2.748} & \textbf{1.312} & \textbf{1.015} & 0.792 \\
%     \bottomrule
%     \end{tabular}%
    \begin{tabular}{llrrrrrr}
    \toprule
    \multirow{2}[4]{*}{\textbf{Complexity}} & \multirow{2}[4]{*}{\textbf{Model}} & \multicolumn{2}{c}{\textbf{ETTh1}} & \multicolumn{2}{c}{\textbf{ETTh2}} & \multicolumn{2}{c}{\textbf{ETTm1}} \\
\cmidrule{3-8}          &       & \multicolumn{1}{c}{\textbf{MSE↓}} & \multicolumn{1}{c}{\textbf{MAE↓}} & \multicolumn{1}{c}{\textbf{MSE↓}} & \multicolumn{1}{c}{\textbf{MAE↓}} & \multicolumn{1}{c}{\textbf{MSE↓}} & \multicolumn{1}{c}{\textbf{MAE↓}} \\
    \midrule
    \midrule
    \multicolumn{8}{c}{\textit{Multivariate}} \\
    \midrule
    \midrule
    $O(m^2+nm)$ & vanilla & 1.257 & 0.905 & 3.548 & 1.652 & 1.028 & 0.813 \\
    \midrule
    \multirow{4}[2]{*}{$O(n+m)$} & ABC   & 1.332 & 0.934 & 3.430 & 1.585 & 1.037 & \textbf{0.784} \\
    \multicolumn{1}{l}{} & Performer & 1.455 & 0.966 & 4.018 & 1.770 & 1.203 & 0.832 \\
          & cosFormer & 1.384 & 0.963 & 3.912 & 1.707 & 1.021 & 0.792 \\
          & AMLP  & \textbf{1.247} & \textbf{0.894} & \textbf{2.748} & \textbf{1.312} & \textbf{1.015} & 0.792 \\
    \midrule
    \midrule
    \multicolumn{8}{c}{\textit{Univariate}} \\
    \midrule
    \midrule
    $O(m^2+nm)$ & vanilla & \textbf{0.251} & \textbf{0.240} & 0.266 & 0.419 & 0.479 & 0.619 \\
    \midrule
    \multirow{4}[2]{*}{$O(n+m)$} & ABC   & 0.357 & 0.522 & 0.294 & 0.44  & 0.430 & 0.586 \\
    \multicolumn{1}{l}{} & Performer & 0.267 & 0.440 & \textbf{0.255} & \textbf{0.411} & \textbf{0.325} & \textbf{0.493} \\
          & cosFormer & 0.311 & 0.483 & 0.276 & 0.426 & 0.408 & 0.568 \\
          & AMLP  & 0.346 & 0.509 & 0.260 & 0.415 & 0.420 & 0.575 \\
    \bottomrule
    \end{tabular}%
  \label{tab:ett_full}%
\end{table}%

\section{Experiment Settings for Efficiency Analysis}
\label{efficiency_analysis_settings}
The simulation experiment evaluates NAR-AMLP efficiency from running time and memory usage with respect to sequence length from 256 to 8,192, compared with AR model and vanilla NAR model.
We simulate the generation process with a single efficient module.
For AR, we test its causal attention, which is its bottleneck in generation.
For AMLP, we use $64$ as the inner dimension with ReLU activation function.
\amlpone~and\amlptwo~shares the same complexity, so we use ``AMLP'' to denote the two variants.
The experiments are performed with batch size $12$ on a single A100 GPU, and the results are repeated with 100 runs.
We remain running latency data ranging from the first quatile and the third quatile among the 100 runs to remove noise.
Finally, the remaining figures are averaged to serve as the final time consumption.

\begin{table}[tbp]
  \centering
  \caption{Hyperparameters of different tasks. }
  \resizebox{1.0\linewidth}{!}{
    \begin{tabular}{lccccc}
    \toprule
    \textbf{Task} & \multicolumn{2}{c}{TTS} & MT    & SR    & LSTF \\
    \midrule
    \textbf{Backbone} & \multicolumn{2}{c}{\begin{tabular}[c]{@{}c@{}}FastSpeech~2/\\ Transformer-TTS\end{tabular}} & Transformer/GLAT & SR    & Informer \\
    \midrule
    \textbf{Batch Size} & \multicolumn{2}{c}{48} & --     & 4     & 32 \\
    \textbf{Number of Steps (epochs)} & \multicolumn{2}{c}{20K} & 100K/300K & 1M    & 6 (epochs) \\
    \textbf{Warmup Steps} & \multicolumn{2}{c}{4K} & 4K    & --     & -- \\
    \textbf{Peak Learning Rate} & \multicolumn{2}{c}{5e-4} & 5e-4  & 1e-4  & 1e-4 \\
    \textbf{Scheduler} & \multicolumn{2}{c}{Inverse Sqrt} & Inverse Sqrt & Linear & Exponential Decay \\
    \textbf{Optimizer} & \multicolumn{2}{c}{AdamW} & AdamW & AdamW & AdamW \\
    \textbf{Adam} & \multicolumn{2}{c}{(0.9, 0.98)} & (0.9, 0.98) & (0.9, 0.999) & (0.9,0.999) \\
    \textbf{Clip Norm} & \multicolumn{2}{c}{5.0} & 5.0   & 0     & 0 \\
    \textbf{Attention Dropout} & \multicolumn{2}{c}{0.1} & 0.3   & 0.2   & 0.05 \\
    \textbf{Weight Decay} & \multicolumn{2}{c}{0.01} & 0.0001 & 0     & 0 \\
    \textbf{Max Tokens} & \multicolumn{2}{c}{--} & 65536 & --     & -- \\
    \textbf{Iteration} & \multicolumn{2}{c}{--} &   --    & --     & 5 \\
    \textbf{Evaluation Checkpoint} & \multicolumn{2}{c}{best} & average last 10 & average last 5  & last \\
    \bottomrule
    \end{tabular}%
    }
  \label{tab:hyperparameters}%
\end{table}%

\begin{table}[tbp]
  \centering
  \vspace{-1mm}
  \caption{Hyperparameters of each attention architecture. }
    \begin{tabular}{llcccc}
    \toprule
    \textbf{Architecture} & \textbf{Hyperparameter} & \textbf{TTS} & \textbf{MT} & \textbf{SR} & \textbf{LSTF} \\
    \midrule
    %vanilla & None &  \multicolumn{4}{c}{--} \\
    local & \texttt{wsize} &  15     & 5     & 15    & 15 \\
    ABC   & \texttt{landmarks} &  64    & 16    & 16    & 16 \\
    AMLP  & \texttt{ffn\_dimension}  & 64    & 16    & 16    & 16 \\
    Performer  & \texttt{approx\_attn\_dim} & 64    & 16    & --    & 16 \\
    %cosFormer & None & \multicolumn{4}{c}{--} \\
    \bottomrule
    \end{tabular}%

  \label{tab:attn_param}%
\end{table}%
\newpage
\section{Experiment Results on MT and TTS}
We report the performance of cosFormer and Performer on TTS (Table~\ref{tab:full_tts_result}) and MT (Table~\ref{tab:full_trans_result}) tasks.
We do not include these results in Table~\ref{tab:fastspeech_result} and Table~\ref{tab:trans_result} because these two models perform far behind other efficient models. 
We show their results here for completeness and fair comparison.
\begin{figure}[ht]
  \centering
\begin{minipage}[htbp]{0.47\textwidth}
  \centering
  % \vspace{-1em}
\makeatletter\def\@captype{table}
    \setlength\aboverulesep{0pt}
  \setlength\belowrulesep{0pt}
  \setlength\cellspacetoplimit{2.5pt}
  \setlength\cellspacebottomlimit{2.5pt}
\caption{Automatic evaluation metric on LJSpeech dataset. All models are trained by ourselves. }
\resizebox{1\linewidth}{!}{
    \begin{tabular}{SlSlScSc}
    \toprule
    \multirow{1}[4]{*}{\vspace{-0.5em}\textbf{Arch}} & \multicolumn{1}{Sl}{\multirow{1}[4]{*}{\vspace{-0.5em}\textbf{Model}}} & \multicolumn{2}{Sc}{\textbf{LJSpeech}} \\
\cmidrule{3-4}          &       & \textbf{MCD}$\downarrow$ & \textbf{MSD}$\downarrow$ \\
    \midrule
    \midrule
    \multicolumn{4}{Sc}{\textit{Complexity: $O(n^2)$ or $O\left((n+m)^2\right)$}} \\
    \midrule
    \midrule
    AR    & Tr-TTS & 4.0953 & 2.1985 \\
    \rowcolor[rgb]{ 1,  0.949,  .9} NAR   & FS2 & 3.4748 & 1.9735 \\
    \midrule
    \midrule
    \multicolumn{4}{Sc}{\textit{Complexity: $O(n+m)$}} \\
    \midrule
    \midrule
    AR   & Tr-TTS (ABC) &  5.1302     & 2.5957 \\
    \rowcolor[rgb]{ 1,  .949,  .9} & FS2 (local) & 3.4189 &	1.9704 \\
     \rowcolor[rgb]{ 1,  .949,  .9} & FS2 (cosFormer) & 3.3998 &	1.9561  \\
     \rowcolor[rgb]{ 1,  .949,  .9} & FS2 (Performer) & 3.4374 &	1.9830   \\
    \rowcolor[rgb]{ 1,  .949,  .9} \multirow{1}[3]{*}{NAR} & FS2 (ABC) & 3.3925 & 1.9658 \\
    \rowcolor[rgb]{ 1,  .949,  .9}       & FS2 (XCA) & 3.5003 & 2.0239 \\
    \rowcolor[rgb]{ 1,  .949,  .9}       & FS2 (gMLP) & 3.4025 & 1.9641 \\
\cmidrule{2-4}    \rowcolor[rgb]{ 1,  .949,  .9}       & FS2 (AMLP) & \textbf{3.3274} & \textbf{1.9396} \\
    \bottomrule
    \end{tabular}%
    }

  \label{tab:full_tts_result}%
\end{minipage}
\hspace{5mm}
\begin{minipage}[htbp]{0.47\textwidth}

\makeatletter\def\@captype{table}
  \setlength\aboverulesep{0pt}
  \setlength\belowrulesep{0pt}
  \setlength\cellspacetoplimit{2.5pt}
  \setlength\cellspacebottomlimit{2.5pt}
  \centering
  
  \caption{BLEU4 scores on WMT14 EN-DE and WMT14 DE-EN dataset. All models for comparison are implemented by ourselves. Subscript figures $\boldsymbol{\Delta}$ denote performance drop comparing with backbone models.
``--'' denotes the attention fails in this dataset.}
\resizebox{1\linewidth}{!}{

    \begin{tabular}{SlSlScSc}
    \toprule
    \multirow{1}[4]{*}{\textbf{Arch}} & \multirow{1}[4]{*}{\textbf{Model}} & \multicolumn{2}{Sc}{\textbf{WMT' 14}} \\
\cmidrule{3-4}          &       & \boldmath{}\textbf{En-De}$_{\boldsymbol{\Delta}}$\unboldmath{} & \boldmath{}\textbf{De-En}$_{\boldsymbol{\Delta}}$\unboldmath{} \\
    \midrule
    \midrule
    \multicolumn{4}{Sc}{\textit{Complexity: $O\left((n+m)^2\right)$}} \\
    \midrule
    \midrule
    AR    & Tr & \textbf{27.38} & \textbf{31.26} \\
    \rowcolor[rgb]{ 1,  .949,  .898} NAR   & GLAT  & $26.24$ & $30.10$ \\
    \midrule
    \midrule
    \multicolumn{4}{Sc}{\textit{Complexity: $O(n)$ or $O(n+m)$}} \\
    \midrule
    \midrule
    \multirow{2}[1]{*}{AR} & Tr (local) & $\text{24.77}_{\text{2.61}}$  & $\text{28.21}_{\text{3.05}}$  \\
          & Tr (ABC) & $\text{25.86}_{\text{1.52}}$ & $\text{29.09}_{\text{2.17}}$ \\
          & \qquad \textit{w/ conv} &  26.38$_{\text{1.00}}$  &  30.04$_{\text{1.22}}$  \\ 
    \rowcolor[rgb]{ 1,  .949,  .898}  & GLAT (local) &  18.19$_{8.05}$     & 21.36$_{\text{8.74}}$ \\
    \rowcolor[rgb]{ 1,  .949,  .898}  & GLAT (cosFormer) &    --   & -- \\
    \rowcolor[rgb]{ 1,  .949,  .898} \multirow{1}[3]{*}{NAR}  & GLAT (Performer) &  17.81$_{\text{8.43}}$     & -- \\
    \rowcolor[rgb]{ 1,  .949,  .898}       & GLAT (ABC) & $\text{21.98}_{\text{4.26}}$ & $\text{24.78}_{\text{5.32}}$ \\
    \cmidrule{2-4}
    \rowcolor[rgb]{ 1,  .949,  .898}       & GLAT (AMLP) & $\text{25.00}_{\text{1.24}}$ & $\text{28.42}_{\text{1.68}}$ \\
    \rowcolor[rgb]{ 1,  .949,  .898}  & \qquad \textit{w/ conv} & 25.98$_{\text{\textbf{0.26}}}$  & 29.61$_{\text{\textbf{0.49}}}$ \\
    \bottomrule
    \end{tabular}%
    }

  \label{tab:full_trans_result}%
\end{minipage}
\end{figure}

\section{Task Description}
We provide the statistics of tasks in Table~\ref{tab:task_statistic}.

\begin{table*}[htbp]
  \centering
  \caption{Task statistics of evaluation metrics, input sequence lengths and backbone neural networks. For encoder-decoder architectures, we show both source and target lengths. ($\dag$) denotes the sequence lengths of encoders and decoders of Tr-TTS. The number of final audio phonemes after the vocoder is 559 as well.}
    \begin{tabular}{lllll}
    \toprule
    \textbf{Task} & \multicolumn{1}{l}{\textbf{Dataset}} & \multicolumn{1}{l}{\textbf{Length}} & \multicolumn{1}{l}{\textbf{Model}} & \multicolumn{1}{l}{\textbf{Metric}} \\
    \midrule
    \multirow{2}[2]{*}{TTS} & \multirow{2}[2]{*}{LJSpeech} & 559   & FastSpeech~2 & \multirow{2}[2]{*}{MCD/MSD} \\
          &       & 100/141$^{\dag}$ & Transformer-TTS &  \\
    \midrule
    \multirow{2}[2]{*}{MT} & \multirow{2}[2]{*}{WMT'14 EN-DE} & \multirow{2}[2]{*}{23/21} & Transformer \& & \multirow{2}[2]{*}{BLEU} \\
          &       &       & GLAT  &  \\
    \midrule
    \multirow{2}[2]{*}{SR} &  \multirow{2}[2]{*}{FFHQ \& CelebA-HQ}  & \multirow{2}[2]{*}{16384} & \multirow{2}[2]{*}{SR3} &  \multirow{2}[2]{*}{PSNR/SSMI} \\
          &  &       &       &  \\
    \midrule
    LSTF  & ETT   & 336/720 & Informer & MSE/MAE \\
    \bottomrule
    \end{tabular}%
  \label{tab:task_statistic}%
\end{table*}%

\section{Hyperparameters of Tasks}
We provide the hyperparameters of each task in Table~\ref{tab:hyperparameters}.
We adopt the same hyperparameter sets for Transformer-TTS and FastSpeech~2, which is referred from \citet{fairseq_s2s}. Following \citet{vaswani2017attention} and \citet{qian2020glancing}, we use the same hyperparameters to train Transformer-base and GLAT, respectively.
We implement Transformer-TTS, FastSpeech~2, GLAT and Transformer with fairseq~\citep{fairseq}.
In ``Evaluation Checkpoint'' of Table~\ref{tab:hyperparameters}, ``last'' denotes that we use the last saved checkpoint to test models. 
``best'' denotes that we use the best checkpoint with the lowest MCD value in the validation set for evaluation.
``average last $n$'' denotes that we create a new checkpoint whose parameters are averaged on the parameters of last $n$ ones and use this new checkpoint for performance comparison.

\begin{table}[tbp]
  \centering
  \caption{Hyperparameters of different tasks. }
  \resizebox{1.0\linewidth}{!}{
    \begin{tabular}{lccccc}
    \toprule
    \textbf{Task} & \multicolumn{2}{c}{TTS} & MT    & SR    & LSTF \\
    \midrule
    \textbf{Backbone} & \multicolumn{2}{c}{\begin{tabular}[c]{@{}c@{}}FastSpeech~2/\\ Transformer-TTS\end{tabular}} & Transformer/GLAT & SR    & Informer \\
    \midrule
    \textbf{Batch Size} & \multicolumn{2}{c}{48} & --     & 4     & 32 \\
    \textbf{Number of Steps (epochs)} & \multicolumn{2}{c}{20K} & 100K/300K & 1M    & 6 (epochs) \\
    \textbf{Warmup Steps} & \multicolumn{2}{c}{4K} & 4K    & --     & -- \\
    \textbf{Peak Learning Rate} & \multicolumn{2}{c}{5e-4} & 5e-4  & 1e-4  & 1e-4 \\
    \textbf{Scheduler} & \multicolumn{2}{c}{Inverse Sqrt} & Inverse Sqrt & Linear & Exponential Decay \\
    \textbf{Optimizer} & \multicolumn{2}{c}{AdamW} & AdamW & AdamW & AdamW \\
    \textbf{Adam} & \multicolumn{2}{c}{(0.9, 0.98)} & (0.9, 0.98) & (0.9, 0.999) & (0.9,0.999) \\
    \textbf{Clip Norm} & \multicolumn{2}{c}{5.0} & 5.0   & 0     & 0 \\
    \textbf{Attention Dropout} & \multicolumn{2}{c}{0.1} & 0.3   & 0.2   & 0.05 \\
    \textbf{Weight Decay} & \multicolumn{2}{c}{0.01} & 0.0001 & 0     & 0 \\
    \textbf{Max Tokens} & \multicolumn{2}{c}{--} & 65536 & --     & -- \\
    \textbf{Iteration} & \multicolumn{2}{c}{--} &   --    & --     & 5 \\
    \textbf{Evaluation Checkpoint} & \multicolumn{2}{c}{best} & average last 10 & average last 5  & last \\
    \bottomrule
    \end{tabular}%
    }
  \label{tab:hyperparameters}%
\end{table}%

\begin{table}[tbp]
  \centering
  \vspace{-1mm}
  \caption{Hyperparameters of each attention architecture. }
    \begin{tabular}{llcccc}
    \toprule
    \textbf{Architecture} & \textbf{Hyperparameter} & \textbf{TTS} & \textbf{MT} & \textbf{SR} & \textbf{LSTF} \\
    \midrule
    %vanilla & None &  \multicolumn{4}{c}{--} \\
    local & \texttt{wsize} &  15     & 5     & 15    & 15 \\
    ABC   & \texttt{landmarks} &  64    & 16    & 16    & 16 \\
    AMLP  & \texttt{ffn\_dimension}  & 64    & 16    & 16    & 16 \\
    Performer  & \texttt{approx\_attn\_dim} & 64    & 16    & --    & 16 \\
    %cosFormer & None & \multicolumn{4}{c}{--} \\
    \bottomrule
    \end{tabular}%

  \label{tab:attn_param}%
\end{table}%
